# Supplementary material for: Towards Accurate Labeling of Android Apps for Reliable Malware Detection
Source: arXiv:2007.00464 source file (2020-07-01)
Supplement: Supplementary file 1 [file appendix.tex]

\appendix
\section*{Appendices}
\addcontentsline{toc}{section}{Appendices}
\renewcommand{\thesubsection}{\Alph{subsection}}

\subsection{Manual Analysis Process}
\label{appendix:reversing}
The following steps depicts the process we adopted to manually analyze and label apps in the \emph{Sampled AndroZoo} and \emph{Sampled AndroZoo 2019} datasets. Given an app ($\alpha$), we:
\begin{enumerate}
	\item install ($\alpha$) on a rooted Android Virtual Device (AVD) containing the \texttt{Xposed} framework and the API call monitoring tool \texttt{droidmon}.
 	\item run and interact with ($\alpha$) on the AVD and monitor the API calls it issues during runtime.
 	\item If app crashes or no malicious behavior is noticed: decompile ($\alpha$) with \texttt{Jadx} and inspect its source code.
 	\item If no traces of malicious code are found, disassemble ($\alpha$) with \texttt{Apktool} and reverse engineer its \texttt{smali} code.
 	\item If no traces of malicious code are found, disassemble the shared object libraries used by ($\alpha$) using \texttt{Gidhra} and inspect \texttt{C/C++} code.
 	\item If no traces of malicious code are found, provisionally deem an app as benign and check \texttt{VirusTotal} regarding the app's status.
 	\item If \texttt{VirusTotal} report gives a total of \emph{zero} positives, deem app as benign. Otherwise, inspect the scanners deeming app as malicious, the label they give to an app (e.g., \texttt{Riskware}), and the details inside the scan report.
 	\item If the aforementioned details reveal malicious behavior, deem as such. Otherwise, deem app as benign.
\end{enumerate}

%\subsection{Correctness Versus Malware Type}
%\label{appendix:correctness_type}
%
%The results in table \ref{tab:correctness} depict the evolution of the overall correctness of the \emph{Drebin} scanners on the \emph{AMD} dataset according to \texttt{VirusTotal} scan reports downloaded on \earliestDate{} and on \latestDate{} along with the correctness per malware type. 
%Focusing solely on the overall correctness rates, it is evident that some scanners are indeed more correct than others (e.g., \texttt{ESET}, \texttt{McAfee}, and \texttt{Sophos}). 
%The following observations can be made upon considering the correctness rates per malware type. 
%Firstly, scanners that have decent overall correctness usually score high correctness rates on all malware types. 
%Secondly, on the one hand, some scanners achieve high correctness rates on the majority of malware types yet struggle with others. 
%For example, \texttt{AVG} and \texttt{Kaspersky} appear to struggle with apps belonging to the \texttt{Adware} malware type (emphasized red). 
%On the other hand, some scanners excel against particular malware types, such as \texttt{BitDefender} and \texttt{ClamAV}, which continue to correctly detect the \texttt{HackerTool} malware type.
%As seen in emboldened green, \texttt{BitDefender} and \texttt{ClamAV} appear to score decent correctness rates on the \texttt{HackerTool} malware type, whilst struggling with all other types.
%Lastly, some scanners, such as \texttt{Panda}, appear to struggle on all malware types, even though some apps in the \emph{AMD} dataset are as old as 2010 \cite{wei2017deep}. 
%
%% from Maat.mining import correctness
%% correctness.getCorrectnessByType(datasetDir, vtReportsDir, groundTruth, hashToTypeMapping) # Only hash to type, not to type and family
%%\bgroup
%%\def\arraystretch{1.1}
%\begin{table*}[]
%\centering
%\caption{The change in the correctness rates of the \emph{Drebin} \texttt{VirusTotal} scanners on apps in the \emph{AMD} dataset between \earliestDate{} and \latestDate{}, grouped by malware type.}
%\label{tab:correctness}
%%\small
%\tiny
%\resizebox{\textwidth}{!}{
%%\begin{tabular}{@{}|c|c|c|c|c|c|c|c|c|c|@{}}
%\begin{tabular}{@{}|c|ccccccccc|@{}}
%\toprule
%\backslashbox{Malware Types}{\emph{Drebin} Scanners} & \texttt{AVG} & \texttt{BitDefender} & \texttt{ClamAV} & \texttt{ESET} & \texttt{F-Secure} & \texttt{Kaspersky} & \texttt{McAfee} & \texttt{Panda} & \texttt{Sophos} \\ \hline
%
%\texttt{Adware} & \textcolor{ACMRed}{\emph{0.01}$\rightarrow$\emph{0.01}} & 0.45$\searrow$0.0 & 0.10$\rightarrow$0.10 & 0.98$\nearrow$0.99 & 0.53$\nearrow$0.99 & \textcolor{ACMRed}{\emph{0.26}$\nearrow$\emph{0.33}} & 0.95$\nearrow$0.99 & \textcolor{ACMOrange}{\underline{0.0}$\rightarrow$\underline{0.0}} & 0.92$\nearrow$0.95 \\ \hline
%
%\texttt{Backdoor} & 0.92$\nearrow$0.93 & 0.97$\searrow$0.1 & 0.61$\rightarrow$0.61 & 0.99$\nearrow$1.0 & 0.89$\nearrow$0.99 & 0.98$\rightarrow$0.98 & 0.99$\rightarrow$0.99 & \textcolor{ACMOrange}{\underline{0.01}$\rightarrow$\underline{0.01}} & 0.98$\nearrow$0.99 \\ \hline
%
%\texttt{HackerTool} & 0.99$\nearrow$1.0 & \textcolor{ACMGreen}{\textbf{0.99$\searrow$0.90}} & \textcolor{ACMGreen}{\textbf{0.91}$\rightarrow$\textbf{0.91}} & \textcolor{ACMRed}{\emph{0.81}$\rightarrow$\emph{0.81}} & 0.89$\nearrow$1.0 & \textcolor{ACMRed}{\emph{0.75}$\rightarrow$\emph{0.75}} & 0.99$\rightarrow$0.99 & \textcolor{ACMOrange}{\underline{0.32}$\rightarrow$\underline{0.32}} & 0.99$\rightarrow$0.99\\ \hline
%
%\texttt{Ransom} & 0.98$\nearrow$0.99 & 0.98$\searrow$0.0 & 0.05$\nearrow$0.06 & 0.99$\nearrow$1.0 & 0.89$\nearrow$1.0 & 0.99$\nearrow$1.0 & 0.99$\nearrow$1.0 & \textcolor{ACMOrange}{\underline{0.0}$\rightarrow$\underline{0.0}} & 0.99$\rightarrow$0.99 \\ \hline
%
%\texttt{Trojan} & 0.84$\rightarrow$0.84 & 0.88$\searrow$0.01 & 0.10$\searrow$0.07 & 0.96$\rightarrow$0.96 & 0.75$\nearrow$1.0 & 0.88$\rightarrow$0.88 & 0.99$\nearrow$1.0 & \textcolor{ACMOrange}{\underline{0.0}$\rightarrow$\underline{0.0}} & 0.97$\nearrow$0.98 \\ \hline
%
%\texttt{Trojan-Banker} & 0.98$\nearrow$0.99 & 0.99$\searrow$0.0 & 0.09$\rightarrow$0.09 & 0.99$\nearrow$1.0 & 0.92$\nearrow$1.0 & 0.99$\rightarrow$0.99 & 0.99$\nearrow$1.0 & \textcolor{ACMOrange}{\underline{0.0}$\rightarrow$\underline{0.0}} & 0.99$\nearrow$1.0 \\ \hline
%
%\texttt{Trojan-Clicker} & 0.96$\nearrow$1.0 & 1.0$\searrow$0.0 & 0.32$\rightarrow$0.32 & 1.0$\rightarrow$1.0 & 0.87$\nearrow$1.0 & 0.96$\searrow$0.90 & 1.0$\rightarrow$1.0 & \textcolor{ACMOrange}{\underline{0.0}$\rightarrow$\underline{0.0}} & 1.0$\rightarrow$1.0 \\ \hline
%
%\texttt{Trojan-Dropper} & 0.98$\nearrow$0.99 & 0.96$\searrow$0.03 & 0.10$\nearrow$0.11 & 0.97$\nearrow$0.99 & 0.80$\nearrow$0.99 & 0.97$\nearrow$0.98 & 0.98$\nearrow$1.0 & \textcolor{ACMOrange}{\underline{0.02}$\rightarrow$\underline{0.0}} & 0.97$\nearrow$0.99 \\ \hline
%
%\texttt{Trojan-SMS} & 0.88$\rightarrow$0.88 & 0.98$\searrow$0.0 & 0.24$\searrow$0.15 & 0.99$\rightarrow$0.99 & 0.88$\nearrow$1.0 & 0.98$\nearrow$0.99 & 0.99$\nearrow$1.0 & \textcolor{ACMOrange}{\underline{0.0}$\rightarrow$\underline{0.0}} & 0.99$\rightarrow$0.99 \\ \hline
%
%\texttt{Trojan-Spy} & 0.05$\nearrow$87 & 1.0$\searrow$0.0 & 0.01$\rightarrow$0.01 & 0.99$\nearrow$1.0 & 0.61$\rightarrow$1.0 & 0.99$\rightarrow$0.99 & 0.99$\nearrow$1.0 & \textcolor{ACMOrange}{\underline{0.0}$\rightarrow$\underline{0.0}} & 0.99$\rightarrow$0.99 \\ \hline
%
%Overall Correctness & 0.34$\nearrow$0.40 & 0.68$\searrow$0.02 & 0.15$\searrow$0.13 & \textbf{0.99}$\nearrow$\textbf{1.0} & 0.66$\nearrow$\textbf{0.99} & 0.57$\nearrow$0.61 & \textbf{0.97}$\nearrow$\textbf{1.0} & \textcolor{ACMOrange}{\underline{0.01}$\rightarrow$\underline{0.01}} & 0.95$\rightarrow$\textbf{0.97} \\ \bottomrule
%\end{tabular}}
%\end{table*}
%\egroup

\subsection{Engineered Features}
\label{appendix:engineered_features}
The following list enumerates the engineered features extracted from the \texttt{VirusTotal} scan reports of apps in the \emph{AMD+GPlay} dataset. The order of features in the list mimics the order of every feature in the feature vector.
\begin{enumerate}
	\item The vedicts (i.e., 1 for malicious, 0 for benign, and -1 for unknown), given by the most correct \texttt{VirusTotal} scanners as of \latestDate{}:
	\item[] 
	\begin{itemize*}
		\item \texttt{Avira}
		%\item \texttt{Babable}
		\item \texttt{CAT-QuickHeal}
		\item \texttt{DrWeb}
		\item \texttt{ESET-NOD32}
		\item \texttt{Fortinet}
		\item \texttt{Ikarus}
		\item \texttt{MAX}
		\item \texttt{McAfee}
		\item \texttt{NANO-Antivirus}
		\item \texttt{Sophos}
		\item \texttt{SymantecMobileInsight}
		%\item \texttt{Trustlook}
	\end{itemize*}
%	\item[]
	\item The age of a scan report in years calculated as the difference between today's date and that of \emph{first\_seen}'s.
	\item The number of times the app was submitted to \texttt{VirusTotal} according to the \emph{times\_submitted} field.
	\item The number of scanners deeming the app as malicious according to the \emph{positives} field.
	\item The total number of scanners that scanned the app according to the \emph{total} field.
	\item The list of permissions requested by the app out of 324 permissions. If a permissions is requested by an app, its corresponding index in the feature vector has a value of 1, and a value of 0 otherwise.
 	\item The list of tags given by \texttt{VirusTotal} to the app out of 32 tags. If a tag is given to an app, its corresponding index in the feature vector has a value of 1, and a value of 0 otherwise.
\end{enumerate}

\subsection{Selected Naive Features}
\label{appendix:selected_naive}
The following list enumerates the selected naive features, viz.\ the verdicts of \texttt{VirusTotal} scanners that train the best performing ML-based labeling strategies. The order of features in the list mimics the order of every feature in the feature vector.

\begin{itemize*}
	\item \texttt{AhnLab-V3}
	\item \texttt{Avira}
	\item \texttt{CAT-QuickHeal}
	\item \texttt{Cyren}
	\item \texttt{DrWeb}
	\item \texttt{ESET-NOD32}
	\item \texttt{F-Secure}
	\item \texttt{Fortinet}
	\item \texttt{Ikarus}
	\item \texttt{K7GW}
%	\item \texttt{Kaspersky}
	\item \texttt{MAX}
	\item \texttt{McAfee}
	\item \texttt{McAfee-GW-Edition}
	\item \texttt{NANO-Antivirus}
%	\item \texttt{Qihoo-360}
	\item \texttt{Sophos}
    \item \texttt{SymantecMobileInsight}
	\item \texttt{Trustlook}    
\end{itemize*}

%\subsection{Homegrown Dataset}
%\label{appendix:homegrown}
%The \texttt{SHA1} hashes, a short description, and the \texttt{VirusTotal} \emph{positives}:\emph{total} fields of apps in the \emph{Homegrown} dataset, as of \latestDate{}.
%\begin{table}[h]
%\centering
%\resizebox{\textwidth}{!}{
%\begin{tabular}{|c|c|c|c|}
%\hline
%\texttt{SHA1} Hash & Description & \texttt{Virustotal} \emph{positives} & \texttt{Virustotal} \emph{total} \\ \hline
%17866baec8c1179264c585934d742a7befa20975 & Encryption-based Ransomware demo app & 0 & 56 \\ \hline
%1b8235f2ad665df5f8632b75a1b466f849654934 & Tapjacking-based tracking app and WiFi password stealer & 0 & 56 \\ \hline
%1c7c935ba48c5db86ff4fd957fedc3e691484c77 & Tapjacking and overlay-based Ransomware demo app & 0 & 56 \\ \hline
%31cf1a7a7f8a3bb6f9fdb45267dcbf9ff449b994 & Repackaged app with encryption-based Ransomware payload & 0 & 56 \\ \hline
%66c16d79db25dc9d602617dae0485fa5ae6e54b2 & Repackaged app with logic-based payload to delete user contacts & \textcolor{ACMRed}{1} & 56 \\ \hline
%691973efb45176862085e4d4e081dfa8750590f7 & Repackaged antiviral software with backdoor & 0 & 55 \\ \hline
%aa0d0f82c0a84b8dfc4ecda89a83f171cf675a9a & Repackaged mail client with obfuscated encryption-based Ransomware & 0 & 52 \\ \hline
%bee87f0ae97b438488cbe351311d5d40ccf8c3e0 & Launcher-based Ransomware demo app & 0 & 56 \\ \hline
%\end{tabular}}
%\end{table}

\subsection{\texttt{BitDefender} and \texttt{Panda} Vs. AMD Apps}
\label{appendix:random_amd}
The \texttt{SHA1} hashes of ten apps randomly sampled from the \emph{AMD} dataset, the number of scanners deeming them as malicious as of \latestDate{}, their malware types, and whether \texttt{BitDefender}'s version 3.3.063 and \texttt{Panda}'s version 3.4.5 managed to detect them. 
\begin{table*}[h]
\centering
\resizebox{\textwidth}{!}{
\begin{tabular}{|c|c|c|c|c|}
\hline
\texttt{SHA1} Hash & \texttt{Virustotal} \emph{positives} & Malware Type & \texttt{BitDefender} & \texttt{Panda} \\ \hline
%9e23535839b38b85c1db221178ff3592376fd7000191de6e861b13ec4e147334,fdf0835597adc16d667b4cbaef0fc3ee76205503,22/61,Adware,Undetected,Undetected
fdf0835597adc16d667b4cbaef0fc3ee76205503 & 22 & \texttt{Adware} &  &  \\ \hline
%ed997f5a357e10e705443a245beb6a3be8e9989c3fb02aa70eb8139661dcab5f,3425e68789614cbda4284169589f7aeab8e28b28,29/61,Trojan-SMS,Detected,Detected
3425e68789614cbda4284169589f7aeab8e28b28 & 29 & \texttt{Trojan-SMS} & \checkmark & \checkmark \\ \hline
%1ec721ac0b4f75eb33c55caae1daa88d10a4a5fcfaf7362ffbafc09ea338fb99,11c8678985aaa5ce4bcd5970a0008b0310c88a7e,35/61,Trojan-SMS,Detected,Detected
11c8678985aaa5ce4bcd5970a0008b0310c88a7e & 35 & \texttt{Trojan-SMS} & \checkmark & \checkmark \\ \hline
%9fe742832a0734fa5a53d7ccd3068f3705c023a499cac637b2a7a19cb473dba0,7693726e8f286d6dd8c115c273637d44c554f19c,28/61,Trojan-Banker,Detected,Undetected
7693726e8f286d6dd8c115c273637d44c554f19c & 28 & \texttt{Trojan-Banker} & \checkmark &  \\ \hline
%7ad48cacd10ca678f02cb47ec35645f13cb5388435b16514f1cb2cb23d4bc56d,a0e7e36eec83339980f056a7af5f36d5dc99809e,33/61,Ransom,Detected,Detected
a0e7e36eec83339980f056a7af5f36d5dc99809e & 33 & \texttt{Ransom} & \checkmark & \checkmark \\ \hline
%f02bffb45e14764e3aafec5761e0f1c05fc631ff351c164284e08828ab29b452,74581e2e0c7b93391574ec8582d274432a4a2838,27/61,Adware,Undetected,Undetected
74581e2e0c7b93391574ec8582d274432a4a2838 & 27 & \texttt{Adware} &  &  \\ \hline
%e42bb43aba579950477e097ece0ad04479dde7a5c7b330ac026fd693ec28adc8,a9a46d346a2ae5a397517c70d249695c6c89632b,19/61,Adware,Undetected,Undetected
a9a46d346a2ae5a397517c70d249695c6c89632b & 19 & \texttt{Adware} &  &  \\ \hline
%b2f0ccefa5110811a5460b1bc2eb6164e57c7d516b1466822ca73f7d342ae5bf,db9603ffa852f1b0aad3f44418db44893db3f726,29/61,Adware,Detected,Undetected
db9603ffa852f1b0aad3f44418db44893db3f726 & 29 & \texttt{Adware} & \checkmark &  \\ \hline
%50aad462a69dad46fc0f43adc368c0274e643f733b7e8f76eaa241b2fc669a13,7f9e6bc600b4a02b5d15a6511a43419d1aa500ff,29/61,Adware,Detected,Undetected
7f9e6bc600b4a02b5d15a6511a43419d1aa500ff & 29 & \texttt{Adware} & \checkmark &  \\ \hline
%b49fabcc57e4cfbf5f8c734376af8f7a12d4602ec715d89b3e9df5937abf2772,d4eb21ae5c2b4b05c0f3ce4e5117c56d9c3746ef,23/61,Adware,Detected,Undetected 
d4eb21ae5c2b4b05c0f3ce4e5117c56d9c3746ef & 23 & \texttt{Adware} & \checkmark &  \\ \hline
\end{tabular}}
\end{table*}


\subsection{Static Features}
\label{appendix:static_features}
%As discussed in section \ref{subsec:probabilistic_classification}, we trained our probabilistic classifiers using numerical features statically extracted from the APK archives of apps in the \emph{Piggybacking} (i.e, \emph{Piggybacked}+\emph{Original}), \emph{AMD}, \emph{Malgenome}, and \emph{GPlay} datasets. 
%In total, each app was represented by a vector of 40 features, which are divided into four categories, namely, basic features, permission-based features, API call features, and miscellaneous features. 
The following list enumerates the numerical features statically extracted from the APK archives of apps in the \emph{AndroZoo 2019}, \emph{Sampled AndroZoo}, and \emph{Sampled AndroZoo 2019} datasets. The order of features in the list mimics the order of every feature in the feature vector.
\begin{itemize}
	\item \textbf{Basic features}:
	\item[]
		\begin{enumerate}
			\item[(1)] Minimum SDK version (supported by the app).
			\item[(2)] Maximum SDK version (supported by the app).
			\item[(3)] Total number of activities.
			\item[(4)] Total number of services.
			\item[(5)] Total number of broadcast receivers.
			\item[(6)] Total number of content providers.
		\end{enumerate}
	\item \textbf{Permission-based features}:
	\item[]
		\begin{enumerate}
			\item[(7)] Total request permissions.
			\item[(8)] Ratio of Android permissions to total permissions.
			\item[(9)] Ratio of Custom permissions to total permissions.
			\item[(10)] Ratio of dangerous permissions to total permissions.
		\end{enumerate}
	\item \textbf{API call features}:
	\item[]
		\begin{enumerate}
			\item[(11)] Total number of classes.
			\item[(12)] Total number of methods.
			\item[(13)-(39)] Count of calls to methods in the following packages:
		\end{enumerate}
		\begin{itemize}
			\item \texttt{android.accounts.AccountManager}
			\item \texttt{android.app.Activity}
			\item \texttt{android.app.DownloadManager}
			\item \texttt{android.app.IntentService}
			\item \texttt{android.content.ContentResolver}
			\item \texttt{android.content.ContextWrapper}
			\item \texttt{android.content.pm.PackageInstaller}
			\item \texttt{android.database.sqlite.SQLiteDatabase} \\
			\item \texttt{android.hardware.Camera}
			\item \texttt{android.hardware.display.DisplayManager}
			\item \texttt{android.location.Location}
			\item \texttt{android.media.AudioRecord}
			\item \texttt{android.media.MediaRecorder}
			\item \texttt{android.net.Network} \\
			\item \texttt{android.net.NetworkInfo}
			\item \texttt{android.net.wifi.WifiInfo}
			\item \texttt{android.net.wifi.WifiManager} \\
			\item \texttt{android.os.PowerManager}
			\item \texttt{android.os.Process}
			\item \texttt{android.telephony.SmsManager} \\
			\item \texttt{android.widget.Toast}
			\item \texttt{dalvik.system.DexClassLoader}
			\item \texttt{dalvik.system.PathClassLoader} \\
			\item \texttt{java.lang.class}
			\item \texttt{java.lang.reflect.Method}
			\item \texttt{java.net.HttpCookie}
			\item \texttt{java.net.URL.openConnection}
		\end{itemize}
	\item \textbf{Miscellaneous features}:
		\begin{enumerate}
			\item[40.] Zero-based index of the compiler used to compile the app from (\texttt{dx}, \texttt{dexmerge}, \texttt{dexlib 1.x}, \texttt{dexlib 2.x}, \texttt{Jack 4.x}, or unknown).
		\end{enumerate}
\end{itemize}

\subsection{Hyper Parameter Estimation}
\label{appendix:hyperparameters}
To train the best random forests that comprise our ML-based labeling strategies \Maat{} uses the techniques of \emph{grid search} and \emph{random search} to estimate the hyper parameters of the trees in those forests. We used 10-Fold Cross Validation to train random forests of 100 decision trees and varied the following parameters as follows:

\begin{itemize}
	\item The criterion used to choose the feature to check to further split the training dataset into malicious and benign apps \texttt{criterion}: $\lbrace gini, entropy\rbrace$
	\item The maximum depth a decision tree is allowed to grow \texttt{max\_depth}: $\lbrace 3, 5, 10, None\rbrace$
	\item The maximum number of features a decision tree is allowed to check upon every split \texttt{max\_features}: $\lbrace 3, 5, 10, None\rbrace$			
	\item The minimum number of samples required to split a node in a tree \texttt{min\_samples\_split}: $\lbrace 2, 3, 10\rbrace$		
	\item If False, the entire dataset is used to train the decision tree instead of bootstrap samples \texttt{bootstrap}: $\lbrace True, False\rbrace$			
\end{itemize}
